# Supplementary material for: Electrostatic interactions in atomistic and machine-learned potentials for polar materials
Source: arXiv:2412.01642 source file (2024-12-02)
Supplement: Supplementary file 1 [file appendix.tex]

\section{Electric field far from the system}

To study if the implementation is correct, we report the electric field far from the system of \ch{BaTiO3} with atoms displaced from their centroids. 
The results converge sufficiently far away from the system, proving that the model correctly describe the long range behavior of the system.

\begin{figure}
	\includegraphics[width=\columnwidth]{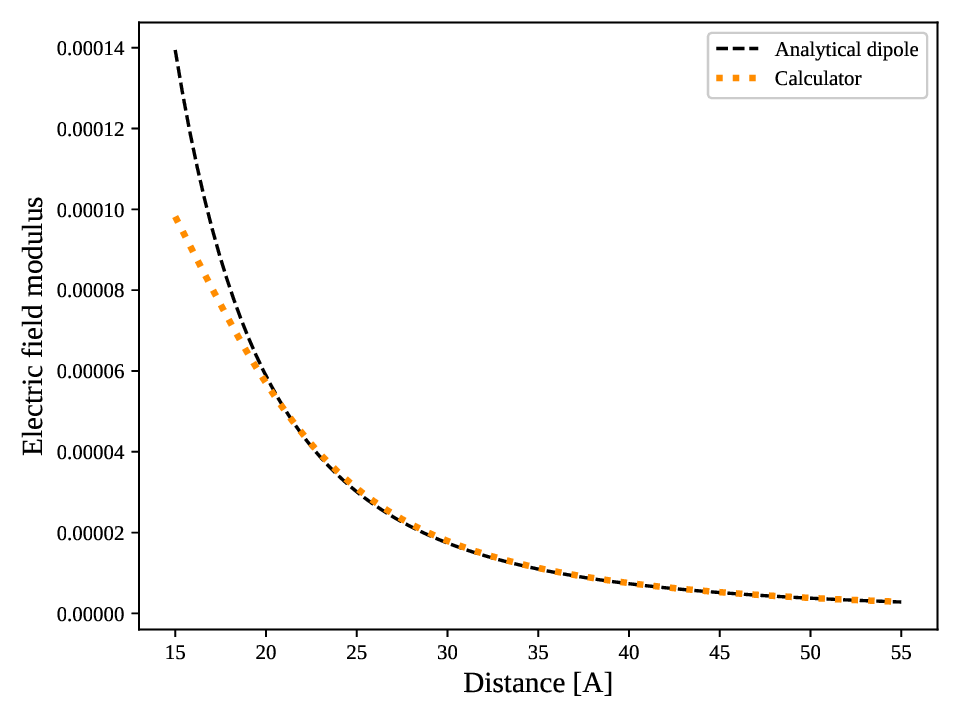}
	\caption{Electric field far from the system (breaking periodic boundary conditions) of the system of charges and from a dipole moment in the origin with the same magnitude as the one obtained from the effective charges.\label{fig:dipole}}
\end{figure}

\section{Dispersion}
To correctly account the long range interaction it is possible to add and subtract the contribution of the force constant computed by electrostatic interactions.
We call $\bPhi^{(sr)}$ the short-range force constant matrix and the $\bPhi^{(lr)}$ the electrostatic force constants matrix computed with the charge model. The short range force constant matrix is defined so that:
\begin{equation}
\bPhi = \bPhi^{(sr)} + \bPhi^{(lr)}
\end{equation}
where $\bPhi$ is the total force-constants matrix.

In \figurename~\ref{fig:disp} we compare the phonon dispersion obtained by Fourier interpolating $\bPhi$ from a 2x2x2 supercell, to the converged one (obtained with the analytical addition of the long-range contribution).
We also plot the result obtained by interpolating to a specific q point the $\bPhi^{(sr)}$ on a 2x2x2 supercell with the $\bPhi^{(lr)}$ on a 4x4x4 supercell.

\begin{figure*}
	\includegraphics[width=\textwidth]{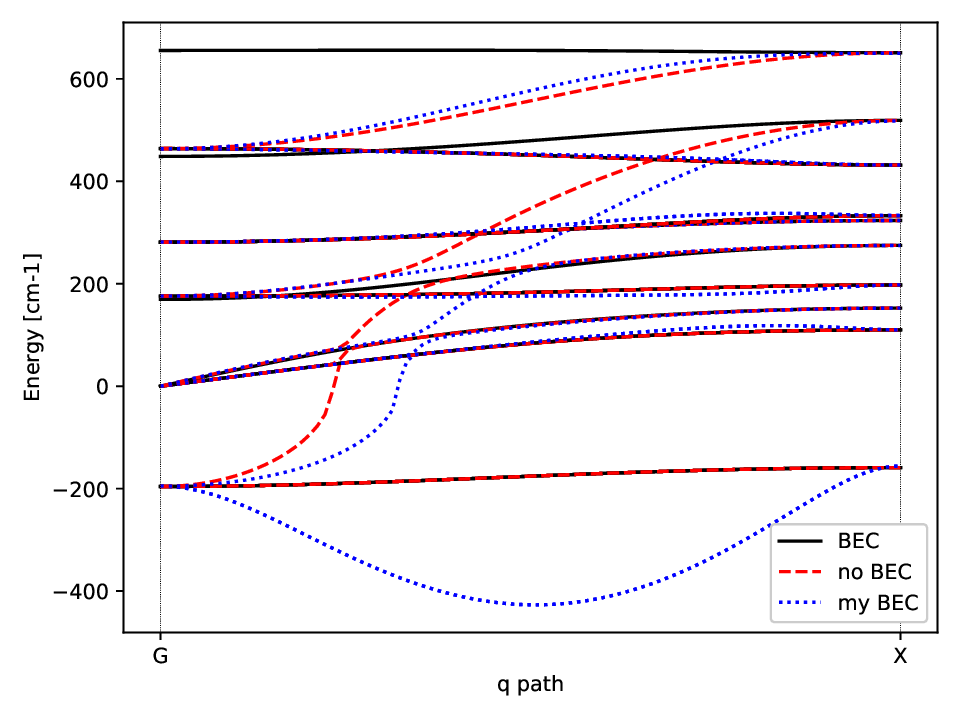}
	\caption{
		Comparison between the exact interpolated value (BEC), the interpolation of the short range $\bPhi$ from a 2x2x2 cell (no BEC), and the separate interpolation of $\bPhi^{(sr)}$ and $\bPhi^{(lr)}$ from a 2x2x2 and a 4x4x4 supercell, respectively (my BEC).
		\label{fig:disp}}
\end{figure*}

The interpolation of $\bPhi^{(lr)}$ is reported in \figurename~\ref{fig:disp:ele}.

\begin{figure*}
	\includegraphics[width=\textwidth]{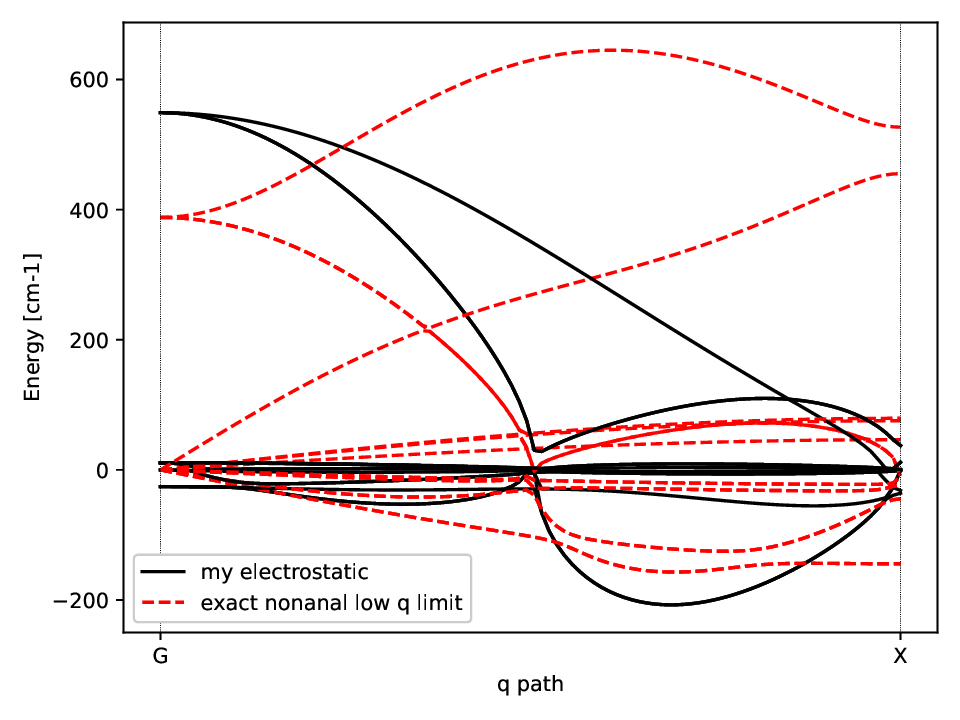}
	\caption{Dispersion of the long-range part of the force constants matrix. This is compared with the analytical expression of the electrostatic forces valid in the low-q limit. Both of them are computed on a 4x4x4 dynamical matrix and then Fourier interpolated (to allow the comparison)\label{fig:disp:ele}}
\end{figure*} 

TODO: Get the dynamical matrix from the non-analytical contribution as it is computed from cellconstructor in the same q-mesh 4x4x4 and compare with those obtained by you. Do the same with the two dispersions and the exact dispersion of long-range interactions.

TODO: Do the analysis computing the two responses very close to gamma, where the low-q limit becomes exact and compare the results.
