# Supplementary material for: Electrostatic interactions in atomistic and machine-learned potentials for polar materials
Source: arXiv:2412.01642 source file (2024-12-02)
Supplement: Supplementary file 2 [file appendix_stress.tex]

\section{Derivation of the stress tensor}
\label{app:stress}

In addition to the vectors in real and reciprocal space from \eqname~\eqref{eq:R:strain} and \eqname~\eqref{eq:k:strain}, the strain tensor $\bm \epsilon$ also change the volume as
\begin{equation}
\Omega' = \Omega\left(1 + \sum_{\alpha\alpha}\varepsilon_{\alpha\alpha}\right).
\end{equation}
The $k^2$ term in the energy changes as
\begin{equation}
{k'}^2 = k^2 - 2\sum_{\alpha\beta}k_\alpha\varepsilon_{\alpha\beta}k_\beta.
\end{equation}
Since $\varepsilon_{\alpha\beta} = \varepsilon_{\beta\alpha}$, the  off-diagonal elements of the stress tensor satisfy the following relation
\begin{equation}
    \frac{d\varepsilon_{\alpha\beta}}{d\varepsilon_{\mu\nu}} =
    \delta_{\alpha\mu}\delta_{\beta\nu} + \delta_{\alpha\nu}\delta_{\beta\mu}. \qquad \mu\neq\nu
\end{equation}
Thus we get:
\begin{subequations}
\begin{equation}
\frac{dR_\alpha}{d\varepsilon_{\mu\nu}} = \delta_{\alpha\mu}R_\nu + \delta_{\alpha\nu}R_\mu
\end{equation}
\begin{equation}
\frac{dk_\alpha}{d\varepsilon_{\mu\nu}} = -\delta_{\alpha\mu}k_\nu - \delta_{\alpha\mu}k_\nu
\end{equation}
\begin{equation}
\frac{dk^2}{d\varepsilon_{\mu\nu}} = -4k_\mu k_\nu
\end{equation}
\begin{equation}
\frac{d\Omega}{d\varepsilon_{\mu\nu}} = \Omega \delta_{\mu\nu}
\end{equation}
\end{subequations}

\begin{widetext}
\begin{align}
\sigma_{\lambda\eta} = &-\frac {1}{\Omega}\sum_{ij\mu\nu\beta}(R_{i\lambda} - \Rcal_{i\lambda})(R_{j\mu} - \Rcal_{j\mu})\frac{Z_{i\beta\eta}Z_{j\nu\mu}}{\Omega}\sum_{\substack{k\\k\neq 0}}\frac{k_\beta k_\nu e^{-\frac{\eta^2k^2}{2}}}{\sum_{\mu\nu} k_\mu\ldielectric_{\mu\nu}k_\nu} e^{-i\bk(\bR_j - \bR_i)} + \nonumber \\ 
&-\frac{1}{\Omega} \sum_{i j\mu\nu\beta}(R_{i\eta} - \Rcal_{i\eta})(R_{j\mu} - \Rcal_{j\mu})\frac{Z_{i\beta\lambda}Z_{j\nu\mu}}{\Omega}\sum_{\substack{k\\k\neq 0}}\frac{k_\beta k_\nu e^{-\frac{\eta^2k^2}{2}}}{\sum_{\mu\nu} k_\mu\ldielectric_{\mu\nu}k_\nu} e^{-i\bk(\bR_j - \bR_i)} + \nonumber \\ 
%& -\frac{1}{2\Omega} \sum_{i\alpha j\nu\beta}(R_{i\alpha} - \Rcal_{i\alpha})(R_{j\lambda} - \Rcal_{j\lambda})\frac{Z_{i\beta\alpha}Z_{j\nu\eta}}{\Omega}\sum_{\substack{k\\k\neq 0}}\frac{k_\beta k_\nu e^{-\frac{\eta^2k^2}{2}}}{\sum_{\mu\nu} k_\mu\ldielectric_{\mu\nu}k_\nu} e^{-i\bk(\bR_j - \bR_i)} + \nonumber \\ 
%&-\frac{1}{2\Omega}  \sum_{i\alpha j\nu\beta}(R_{i\alpha} - \Rcal_{i\alpha})(R_{j\eta} - \Rcal_{j\eta})\frac{Z_{i\beta\alpha}Z_{j\nu\lambda}}{\Omega}\sum_{\substack{k\\k\neq 0}}\frac{k_\beta k_\nu e^{-\frac{\eta^2k^2}{2}}}{\sum_{\mu\nu} k_\mu\ldielectric_{\mu\nu}k_\nu} e^{-i\bk(\bR_j - \bR_i)} + \nonumber \\ 
&+\frac{1}{\Omega}  \sum_{i\alpha j\mu\beta}(R_{i\alpha} - \Rcal_{i\alpha})(R_{j\mu} - \Rcal_{j\mu})\frac{Z_{i\beta\alpha}Z_{j\eta\mu}}{\Omega}\sum_{\substack{k\\k\neq 0}}\frac{k_\beta k_\lambda e^{-\frac{\eta^2k^2}{2}}}{\sum_{\mu\nu} k_\mu\ldielectric_{\mu\nu}k_\nu} e^{-i\bk(\bR_j - \bR_i)} + \nonumber \\ 
&+\frac{1}{\Omega} \sum_{i\alpha j\mu\beta}(R_{i\alpha} - \Rcal_{i\alpha})(R_{j\mu} - \Rcal_{j\mu})\frac{Z_{i\beta\alpha}Z_{j\lambda\mu}}{\Omega}\sum_{\substack{k\\k\neq 0}}\frac{k_\beta k_\eta e^{-\frac{\eta^2k^2}{2}}}{\sum_{\mu\nu} k_\mu\ldielectric_{\mu\nu}k_\nu} e^{-i\bk(\bR_j - \bR_i)} + \nonumber \\ 
%& +\frac{1}{2\Omega}\sum_{i\alpha j\mu\nu}(R_{i\alpha} - \Rcal_{i\alpha})(R_{j\mu} - \Rcal_{j\mu})\frac{Z_{i\eta\alpha}Z_{j\nu\mu}}{\Omega}\sum_{\substack{k\\k\neq 0}}\frac{k_\lambda k_\nu e^{-\frac{\eta^2k^2}{2}}}{\sum_{\mu\nu} k_\mu\ldielectric_{\mu\nu}k_\nu} e^{-i\bk(\bR_j - \bR_i)} + \nonumber \\ 
%& +\frac{1}{2\Omega}\sum_{i\alpha j\mu\nu}(R_{i\alpha} - \Rcal_{i\alpha})(R_{j\mu} - \Rcal_{j\mu})\frac{Z_{i\lambda\alpha}Z_{j\nu\mu}}{\Omega}\sum_{\substack{k\\k\neq 0}}\frac{k_\eta k_\nu e^{-\frac{\eta^2k^2}{2}}}{\sum_{\mu\nu} k_\mu\ldielectric_{\mu\nu}k_\nu} e^{-i\bk(\bR_j - \bR_i)} + \nonumber \\ 
&-\frac{\eta^2}{\Omega} \sum_{i\alpha j\mu\nu\beta}(R_{i\alpha} - \Rcal_{i\alpha})(R_{j\mu} - \Rcal_{j\mu})\frac{Z_{i\beta\alpha}Z_{j\nu\mu}}{\Omega}\sum_{\substack{k\\k\neq 0}}\frac{k_\beta k_\nu k_\lambda k_\eta e^{-\frac{\eta^2k^2}{2}}}{\sum_{\mu\nu} k_\mu\ldielectric_{\mu\nu}k_\nu} e^{-i\bk(\bR_j - \bR_i)} + \nonumber \\ 
&-\frac{1}{\Omega}\sum_{i\alpha j\mu\nu\beta\gamma}(R_{i\alpha} - \Rcal_{i\alpha})(R_{j\mu} - \Rcal_{j\mu})\frac{Z_{i\beta\alpha}Z_{j\nu\mu}}{\Omega}\sum_{\substack{k\\k\neq 0}}\frac{k_\beta k_\nu (k_\lambda\epsilon_{\eta\gamma} + k_\eta \epsilon_{\lambda\gamma})k_\gamma e^{-\frac{\eta^2k^2}{2}}}{(\sum_{\mu\nu} k_\mu\ldielectric_{\mu\nu}k_\nu)^2} e^{-i\bk(\bR_j - \bR_i)}  + \nonumber \\
&+\delta_{\lambda\eta}\frac{\mathcal E}{\Omega}% \sum_{i\alpha j\mu\nu\beta}(R_{i\alpha} - \Rcal_{i\alpha})(R_{j\mu} - \Rcal_{j\mu})\frac{Z_{i\beta\alpha}Z_{j\nu\mu}}{\Omega}\sum_{\substack{k\\k\neq 0}}\frac{k_\beta k_\nu e^{-\frac{\eta^2k^2}{2}}}{\sum_{\mu\nu} k_\mu\ldielectric_{\mu\nu}k_\nu} e^{-i\bk(\bR_j - \bR_i)} 
\label{eq:stress}
\end{align}
\end{widetext}
